# Supplementary material for: STATrack: A Target-Aware Fully Spiking Neural Network for Efficient UAV Tracking
Source: arXiv:2603.27493 source file (2026-08-26)
Supplement: Supplementary file 1 [file Appendix.tex]

\documentclass[a4paper,fleqn]{cas-sc}

\usepackage{booktabs}
\usepackage{longtable}
\usepackage{multirow}
\usepackage{makecell}
\usepackage{graphicx}
\usepackage{xcolor}
\usepackage{amsmath}
\usepackage{amssymb}

\begin{document}

\shorttitle{Fully Spiking Neural Networks with Target Awareness for Energy-Efficient UAV Tracking}
\shortauthors{Zhong et al.}
\title[mode=title]{\textbf{Fully Spiking Neural Networks with Target Awareness for Energy-Efficient UAV Tracking}\\
Supplementary Material}

\begin{abstract}
 Spiking Neural Networks (SNNs), characterized by their event-driven computation and low power consumption, have shown great potential for energy-efficient visual tracking on unmanned aerial vehicles (UAVs). However, existing SNN-based trackers often rely on costly event cameras, which limits their deployment on standard RGB-camera UAV platforms. To address this limitation, we propose STATrack, a fully spiking neural network framework for UAV visual tracking using only RGB inputs. To the best of our knowledge, this is the first study to explore fully spiking neural networks for RGB-based UAV visual tracking. To alleviate target semantic degradation caused by spike discretization and reduce background interference in UAV scenes, we introduce an Adaptive Mutual Information Maximization (AMIM) mechanism. AMIM maximizes the mutual information between template inputs and their deep target-aware features, encouraging the spiking backbone to preserve discriminative target semantics. In addition, a sample-difficulty-aware dynamic weighting strategy is designed to adaptively adjust the mutual information constraint during training. Extensive experiments on four widely used UAV tracking benchmarks demonstrate that STATrack achieves state-of-the-art tracking performance with low theoretical energy consumption, highlighting its potential for energy-constrained UAV applications. Code is released at: \href{https://anonymous.4open.science/r/STATrack}{https://anonymous.4open.science/r/STATrack}.
\end{abstract}

\begin{keywords}
Spiking Neural Network \sep Mutual Information \sep UAV Tracking \sep Energy-Efficient Vision
\end{keywords}
\maketitle

\section{Global Statistics Network}
\label{sec:supp_gsn}

The global statistics network \(T_{\theta}(\cdot)\) is implemented as a lightweight multi-layer perceptron (MLP) to estimate the statistical dependency between the template input and its target-aware feature representation. Given a feature map \(\mathbf{Z} \in \mathbb{R}^{B \times C \times H \times W}\) and its associated representation \(\mathbf{t}_{Z} \in \mathbb{R}^{B \times d_{\mathrm{rep}}}\), both extracted from the same template image, the network first downsamples \(\mathbf{Z}\) to a fixed spatial resolution using adaptive average pooling:
\begin{equation}
\tilde{\mathbf{Z}} 
= 
\mathrm{AAP}_{16 \times 16}(\mathbf{Z})
\in \mathbb{R}^{B \times C \times 16 \times 16},
\label{eq:supp_aap}
\end{equation}
where \(\mathrm{AAP}_{16 \times 16}(\cdot)\) denotes adaptive average pooling with output size \(16 \times 16\). The pooled feature map and the target-aware representation are then flattened and concatenated:
\begin{equation}
\mathbf{h}_0 =
\left[
\mathrm{Flatten}(\tilde{\mathbf{Z}})\; \big|\;
\mathrm{Flatten}(\mathbf{t}_{Z})
\right]
\in \mathbb{R}^{B \times d_{\mathrm{in}}},
\label{eq:supp_concat}
\end{equation}
where the input dimension is defined as:
\begin{equation}
d_{\mathrm{in}} = 256 \times C + d_{\mathrm{rep}}.
\label{eq:supp_din}
\end{equation}

The concatenated vector \(\mathbf{h}_0\) is passed through a three-layer MLP to produce a scalar statistics score:
\begin{align*}
&\mathbf{h}_1 = \mathrm{ReLU}(\mathbf{W}_1 \mathbf{h}_0 + \mathbf{b}_1), \\
&\mathbf{h}_2 = \mathrm{ReLU}(\mathbf{W}_2 \mathbf{h}_1 + \mathbf{b}_2), \\
&T_{\theta}(\mathbf{Z}, \mathbf{t}_{Z}) = \mathbf{W}_3 \mathbf{h}_2 + \mathbf{b}_3.
\end{align*}
where \(\mathbf{W}_1 \in \mathbb{R}^{512 \times d_{\mathrm{in}}}\), \(\mathbf{b}_1 \in \mathbb{R}^{512}\), \(\mathbf{W}_2 \in \mathbb{R}^{128 \times 512}\), \(\mathbf{b}_2 \in \mathbb{R}^{128}\), \(\mathbf{W}_3 \in \mathbb{R}^{1 \times 128}\), and \(\mathbf{b}_3 \in \mathbb{R}\). The scalar output \(T_{\theta}(\mathbf{Z}, \mathbf{t}_{Z})\) serves as the critic score in the Jensen--Shannon divergence-based mutual information estimator.
\section{Layer-wise Spike Firing Rate}
\label{sec:supp_firing_rate}

This section reports the layer-wise spike firing rates of STATrack and STATrack-s. 

\begin{longtable}{cccccc}
\caption{Layer-wise firing rates of STATrack and STATrack-s.}\label{tab:firing_details} \\
\toprule
\textbf{Stage} & \textbf{Module} & \textbf{Submodule} & \textbf{Layer} & \textbf{STATrack} & \textbf{STATrack-s} \\
\midrule
\endfirsthead
\multicolumn{6}{c}{\tablename~\thetable{} -- continued from previous page} \\
\toprule
\textbf{Stage} & \textbf{Module} & \textbf{Submodule} & \textbf{Layer} & \textbf{STATrack} & \textbf{STATrack-s} \\
\midrule
\endhead
\midrule
\multicolumn{6}{r}{Continued on next page} \\
\endfoot
\bottomrule
\endlastfoot
\multirow{6}{*}{\textbf{Stage 1}} & \multicolumn{2}{c}{Downsampling} & Conv & 1.0000 & 1.0000 \\ \cmidrule(lr){2-6}
 & \multirow{5}{*}{\makecell{Conv-Based\\SNN Block}} & \multirow{3}{*}{SSConv} & PWConv1 & 0.3738 & 0.3333 \\
 &  &  & DWConv & 0.3613 & 0.3301 \\
 &  &  & PWConv2 & 0.3820 & 0.3584 \\ \cmidrule(lr){3-6}
 &  & \multirow{2}{*}{ChConv} & Conv1 & 0.3588 & 0.4436 \\
 &  &  & Conv2 & 0.0698 & 0.1102 \\ \midrule
\multirow{6}{*}{\textbf{Stage 2}} & \multicolumn{2}{c}{Downsampling} & Conv & 0.3008 & 0.3093 \\ \cmidrule(lr){2-6}
 & \multirow{5}{*}{\makecell{Conv-Based\\SNN Block}} & \multirow{3}{*}{SSConv} & PWConv1 & 0.2129 & 0.2367 \\
 &  &  & DWConv & 0.2734 & 0.2911 \\
 &  &  & PWConv2 & 0.1879 & 0.1990 \\ \cmidrule(lr){3-6}
 &  & \multirow{2}{*}{ChConv} & Conv1 & 0.3006 & 0.3574 \\
 &  &  & Conv2 & 0.0418 & 0.0535 \\ \midrule
\multirow{11}{*}{\textbf{Stage 3}} & \multicolumn{2}{c}{Downsampling} & Conv & 0.2831 & 0.3126 \\ \cmidrule(lr){2-6}
 & \multirow{5}{*}{\makecell{Conv-Based\\SNN Block 1}} & \multirow{3}{*}{SSConv} & PWConv1 & 0.2307 & 0.2139 \\
 &  &  & DWConv & 0.2526 & 0.2638 \\
 &  &  & PWConv2 & 0.1518 & 0.1768 \\ \cmidrule(lr){3-6}
 &  & \multirow{2}{*}{ChConv} & Conv1 & 0.2460 & 0.2666 \\
 &  &  & Conv2 & 0.0269 & 0.0325 \\ \cmidrule(lr){2-6}
 & \multirow{5}{*}{\makecell{Conv-Based\\SNN Block 2}} & \multirow{3}{*}{SSConv} & PWConv1 & 0.3447 & 0.3848 \\
 &  &  & DWConv & 0.1834 & 0.1872 \\
 &  &  & PWConv2 & 0.1251 & 0.1544 \\ \cmidrule(lr){3-6}
 &  & \multirow{2}{*}{ChConv} & Conv1 & 0.2407 & 0.2863 \\
 &  &  & Conv2 & 0.0206 & 0.0277 \\ \midrule
\multirow{55}{*}{\textbf{Stage 4}} & \multicolumn{2}{c}{Downsampling} & Conv & 0.3105 & 0.3414 \\ \cmidrule(lr){2-6}
 & \multirow{9}{*}{\makecell{Transformer-Based\\SNN Block 1}} & \multirow{3}{*}{SSConv} & PWConv1 & 0.1932 & 0.2222 \\
 &  &  & DWConv & 0.2293 & 0.2674 \\
 &  &  & PWConv2 & 0.0864 & 0.1028 \\ \cmidrule(lr){3-6}
 &  & \multirow{6}{*}{E-SDSA} & $Q_S$ & 0.2280 & 0.2676 \\
 &  &  & $K_S$ & 0.2280 & 0.2676 \\
 &  &  & $V_S$ & 0.2280 & 0.2676 \\
 &  &  & $Q_S K_S^T$ & 0.0283 & 0.0282 \\
 &  &  & Context & 0.1647 & 0.1490 \\
 &  &  & Linear & 0.6407 & 0.5747 \\ \cmidrule(lr){2-6}
 & \multirow{9}{*}{\makecell{Transformer-Based\\SNN Block 2}} & \multirow{3}{*}{SSConv} & PWConv1 & 0.3531 & 0.4023 \\
 &  &  & DWConv & 0.1954 & 0.2285 \\
 &  &  & PWConv2 & 0.1135 & 0.1270 \\ \cmidrule(lr){3-6}
 &  & \multirow{6}{*}{E-SDSA} & $Q_S$ & 0.3447 & 0.3738 \\
 &  &  & $K_S$ & 0.3447 & 0.3738 \\
 &  &  & $V_S$ & 0.3447 & 0.3738 \\
 &  &  & $Q_S K_S^T$ & 0.0113 & 0.0122 \\
 &  &  & Context & 0.0938 & 0.0677 \\
 &  &  & Linear & 0.5173 & 0.4281 \\ \cmidrule(lr){2-6}
 & \multirow{9}{*}{\makecell{Transformer-Based\\SNN Block 3}} & \multirow{3}{*}{SSConv} & PWConv1 & 0.3928 & 0.4141 \\
 &  &  & DWConv & 0.2197 & 0.2300 \\
 &  &  & PWConv2 & 0.1209 & 0.1191 \\ \cmidrule(lr){3-6}
 &  & \multirow{6}{*}{E-SDSA} & $Q_S$ & 0.3740 & 0.3773 \\
 &  &  & $K_S$ & 0.3740 & 0.3773 \\
 &  &  & $V_S$ & 0.3740 & 0.3773 \\
 &  &  & $Q_S K_S^T$ & 0.0102 & 0.0114 \\
 &  &  & Context & 0.0780 & 0.0510 \\
 &  &  & Linear & 0.4910 & 0.4093 \\ \cmidrule(lr){2-6}
 & \multirow{9}{*}{\makecell{Transformer-Based\\SNN Block 4}} & \multirow{3}{*}{SSConv} & PWConv1 & 0.3541 & 0.4153 \\
 &  &  & DWConv & 0.1851 & 0.2305 \\
 &  &  & PWConv2 & 0.1079 & 0.1349 \\ \cmidrule(lr){3-6}
 &  & \multirow{6}{*}{E-SDSA} & $Q_S$ & 0.3363 & 0.3988 \\
 &  &  & $K_S$ & 0.3363 & 0.3988 \\
 &  &  & $V_S$ & 0.3363 & 0.3988 \\
 &  &  & $Q_S K_S^T$ & 0.0069 & 0.0100 \\
 &  &  & Context & 0.0541 & 0.0370 \\
 &  &  & Linear & 0.2270 & 0.2993 \\ \cmidrule(lr){2-6}
 & \multirow{9}{*}{\makecell{Transformer-Based\\SNN Block 5}} & \multirow{3}{*}{SSConv} & PWConv1 & 0.3146 & 0.3835 \\
 &  &  & DWConv & 0.1861 & 0.2350 \\
 &  &  & PWConv2 & 0.0950 & 0.1153 \\ \cmidrule(lr){3-6}
 &  & \multirow{6}{*}{E-SDSA} & $Q_S$ & 0.2832 & 0.3577 \\
 &  &  & $K_S$ & 0.2832 & 0.3577 \\
 &  &  & $V_S$ & 0.2832 & 0.3577 \\
 &  &  & $Q_S K_S^T$ & 0.0111 & 0.0100 \\
 &  &  & Context & 0.0780 & 0.0491 \\
 &  &  & Linear & 0.3731 & 0.2999 \\ \cmidrule(lr){2-6}
 & \multirow{9}{*}{\makecell{Transformer-Based\\SNN Block 6}} & \multirow{3}{*}{SSConv} & PWConv1 & 0.2650 & 0.3335 \\
 &  &  & DWConv & 0.1820 & 0.2277 \\
 &  &  & PWConv2 & 0.0847 & 0.1163 \\ \cmidrule(lr){3-6}
 &  & \multirow{6}{*}{E-SDSA} & $Q_S$ & 0.2197 & 0.2911 \\
 &  &  & $K_S$ & 0.2197 & 0.2911 \\
 &  &  & $V_S$ & 0.2197 & 0.2911 \\
 &  &  & $Q_S K_S^T$ & 0.0096 & 0.0089 \\
 &  &  & Context & 0.0897 & 0.0532 \\
 &  &  & Linear & 0.3643 & 0.3075 \\ \midrule
\multirow{19}{*}{\textbf{Stage 5}} & \multicolumn{2}{c}{Downsampling} & Conv & 0.1703 & 0.2274 \\ \cmidrule(lr){2-6}
 & \multirow{9}{*}{\makecell{Transformer-Based\\SNN Block 1}} & \multirow{3}{*}{SSConv} & PWConv1 & 0.1555 & 0.2177 \\
 &  &  & DWConv & 0.0841 & 0.1225 \\
 &  &  & PWConv2 & 0.0878 & 0.0944 \\ \cmidrule(lr){3-6}
 &  & \multirow{6}{*}{E-SDSA} & $Q_S$ & 0.2249 & 0.2816 \\
 &  &  & $K_S$ & 0.2249 & 0.2816 \\
 &  &  & $V_S$ & 0.2249 & 0.2816 \\
 &  &  & $Q_S K_S^T$ & 0.0065 & 0.0071 \\
 &  &  & Context & 0.0138 & 0.0185 \\
 &  &  & Linear & 0.0700 & 0.1064 \\ \cmidrule(lr){2-6}
 & \multirow{9}{*}{\makecell{Transformer-Based\\SNN Block 2}} & \multirow{3}{*}{SSConv} & PWConv1 & 0.2920 & 0.2866 \\
 &  &  & DWConv & 0.0397 & 0.0413 \\
 &  &  & PWConv2 & 0.0557 & 0.0495 \\ \cmidrule(lr){3-6}
 &  & \multirow{6}{*}{E-SDSA} & $Q_S$ & 0.2218 & 0.2354 \\
 &  &  & $K_S$ & 0.2218 & 0.2354 \\
 &  &  & $V_S$ & 0.2218 & 0.2354 \\
 &  &  & $Q_S K_S^T$ & 0.0100 & 0.0040 \\
 &  &  & Context & 0.0152 & 0.0056 \\
 &  &  & Linear & 0.2141 & 0.0604 \\ \midrule
\multirow{15}{*}{\textbf{Head}} & \multirow{5}{*}{Ctr} & -- & Conv1 & 0.1244 & 0.1894 \\
 &  & -- & Conv2 & 0.0666 & 0.0658 \\
 &  & -- & Conv3 & 0.1026 & 0.0636 \\
 &  & -- & Conv4 & 0.2131 & 0.1114 \\
 &  & -- & Conv5 & 0.2131 & 0.1114 \\ \cmidrule(lr){2-6}
 & \multirow{5}{*}{Offset} & -- & Conv1 & 0.1244 & 0.1894 \\
 &  & -- & Conv2 & 0.0568 & 0.0566 \\
 &  & -- & Conv3 & 0.0802 & 0.0916 \\
 &  & -- & Conv4 & 0.0801 & 0.0812 \\
 &  & -- & Conv5 & 0.0801 & 0.0812 \\ \cmidrule(lr){2-6}
 & \multirow{5}{*}{Size} & -- & Conv1 & 0.1244 & 0.1894 \\
 &  & -- & Conv2 & 0.0701 & 0.0722 \\
 &  & -- & Conv3 & 0.1052 & 0.0985 \\
 &  & -- & Conv4 & 0.1809 & 0.1390 \\
 &  & -- & Conv5 & 0.1809 & 0.1390 \\
\end{longtable}

\end{document}
